# Supplementary material for: Highly-Efficient Persistent FIFO Queues
Source: arXiv:2402.17674 source file (2024-12-10)
Supplement: Supplementary file 1 [file appendix.tex]

\begin{subappendices}

\section{Proof of Lemma~\ref{lin_deq}} \label{sec:lemma-proof}
\begin{proof}
Since $\var{deq}$ is persisted, 
either a value of \Head\ greater than $i$ has been written back
by $c_k$, or an index with value at least $i+R$ has been written into $\Q$ 
and into NVM by $c_k$. 

In case (a), 
\Head\ has a value greater than $i$ at the beginning of the execution of the recovery code. 
By inspection of the code, \Head\ is not assigned a value smaller than this initial value. 
In the second case, let $m$ be the index, which is greater than or equal to $i+R$. 
That index has been written by a \CAS\ of line~\ref{pcrq:dqtran} or~\ref{pcrq:empty-1} 
into $\Q$, and it has been written back by $c_k$. We argue that a greater value than $m-R$ will be 
written into \Head\ during the execution of lines~\ref{pcrq:recinimax}-\ref{pcrq:rec-max-found}.
By inspection of the recovery code, $\Tail$ gets a value greater than the maximum index in elements of $Q$
at recovery time. Thus, $\Tail$ has a value greater than $m-R$, because of 
lines~\ref{pcrq:rec-tail-emptychk}-\ref{pcrq:rec-tail-set1}. Due to 
lines~\ref{pcrq:recinimax}-\ref{pcrq:rec-max-found},
$\Head$ will be initialized to a value greater than $m-R$. After recovery, $\Head$ has a value 
greater than $i$.
This proves case (a).

In case (b),
because $\var{deq}$ is persisted, either some value of $\Head > i$ has been written back 
by $c_k$ or a value $\var{idx}\geq i$ has been written in some element of $\Q$ and in NVM by $c_k$.
Assume first that a value of $\Head > i$ has been written back by $c_k$.
It is apparent from lines~\ref{pcrq:recemptycheck}-\ref{pcrq:rec-min-found}, that 
$\Tail \geq \Head$, at recovery time. Thus,
\Tail\ has a value at least $i$ at recovery time.
The other case is also simple. By inspection of Algorithm~\ref{alg:pcrq}, if at some point in time,
an element of $\Q$ stores an index $\var{idx}$, then it will store an index at least as large as 
$\var{idx}$ at all later times. 
At recovery time, \Tail\ gets the maximum among all indices
written in $Q$, and by assumption, a value greater than or equal to $i$
has been written in some element of $Q$ and persisted by $c_k$. \qed
\end{proof}

\section{Counter examples} \label{sec:counter-examples}

\remove{
\begin{scenario} \label{scn:piq-head-counter}
Assume there is an enqueue operation $\var{enq}_j(x)$ which is persisted and thus it is linearized. 
Assume that the matching dequeue 
$\var{deq}_j$ has not persisted $\top$ in $\Q$ and there exists a following 
$\var{deq}_{j'},\: j'>j$, in $E_k$ which is 
persisted. Since $\var{enq}_j$ is persisted, $\var{deq}_j$ will be assigned a linearization point 
(by the linearization scheme described above). If \Head\ is set to point to $j$ or to some smaller index, then 
$x$ will be dequeued again by some other dequeue in the future, which is incorrect. Note also that 
not linearizing 
$\var{deq}_j$ is not a solution for the following reason. Assume that $\var{enq}_j$ has been 
completed, and thus it has 
to be linearized to ensure durable linearizability. After the completion of $\var{enq}_j$, assume 
that another enqueue 
operation is executed that writes $x'$ in $\Q[j']$, where $j'>j$. Let $\var{deq}_{j'}$ be the matching dequeue of 
$\var{enq}_{j'}$,  and let $\var{deq}_{j'}$ complete before the crash. If we do not linearize 
$\var{deq}_j$, then the 
\FIFO\ property is violated. Thus, we have to linearize $\var{deq}_j$ despite the fact that it is 
not a persisted operation.
\end{scenario}

\begin{figure}[htb]
\centering
\includegraphics{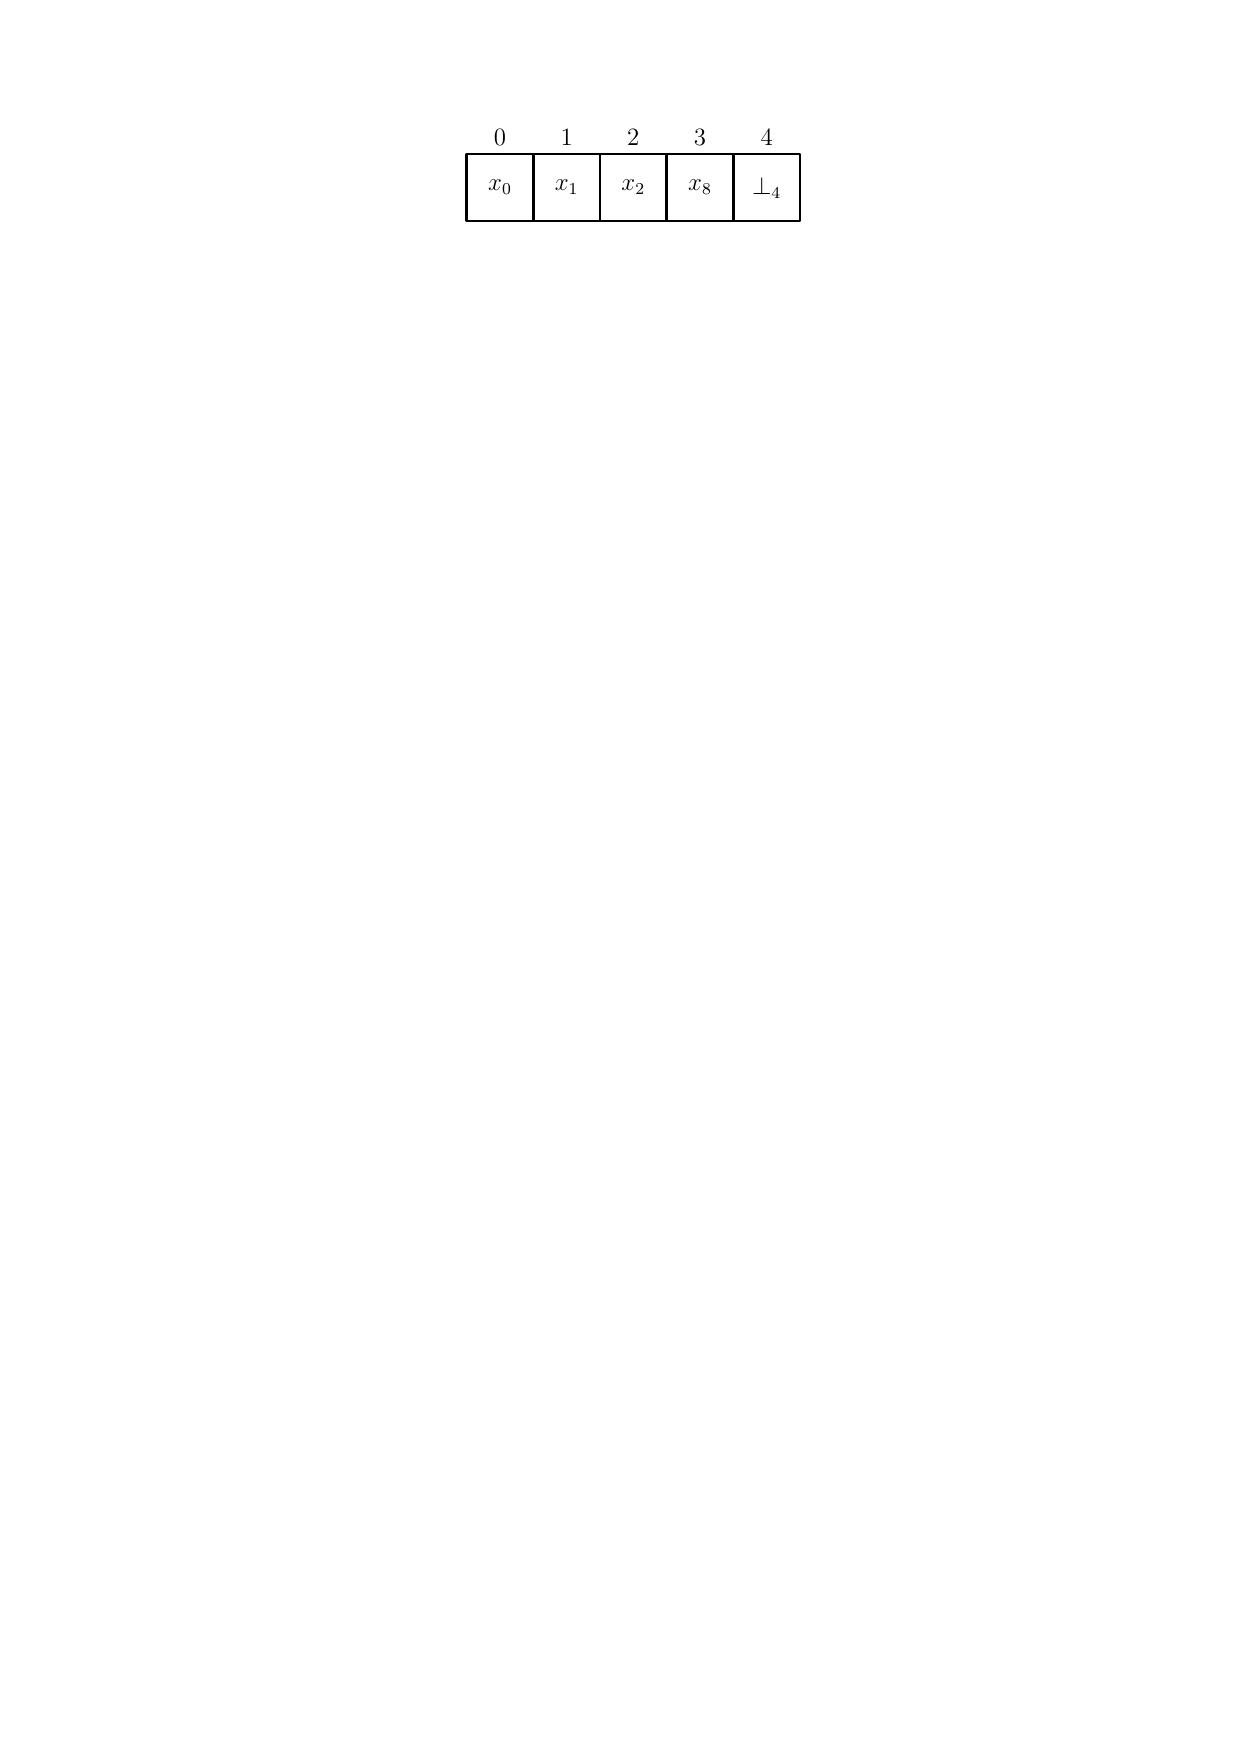}
\caption{\PCRQ\ uncertainty problem. The subscript at each value indicates
the triplet's index field.} \label{fig:crqunc}
\end{figure}

\begin{scenario} \label{scn:uncertaintyProblem-full}
Let the state of the circular array $\crqVar.\Q$ of size $R=5$ be the one shown in the top part 
of Figure~\ref{fig:crqunc} after some crash $c_k$.
There are four items $x_0, \ldots, x_2$ and $x_8$ in $\crqVar.\Q$.
A hypothetical infinite array $\HypQ$ is also shown in the bottom part of Figure~\ref{fig:crqunc}.
We assign each item to its respective position at $\HypQ$.
For example, item $x_2$ is placed at position $2$ in
$\HypQ$, while $x_8$ is placed at position $8$ in $\HypQ$, which corresponds to position $3$ in 
$\crqVar.\Q$ because $8\bmod 5 = 3$.
Notice that $\HypQ[5]$ up to $\HypQ[7]$, and from $\HypQ[9]$ and on there are no items.
The items that were going to be inserted there (if they existed) were not written back to NVM,
either by a \pwbi-\psynci\ pair or by a system eviction. Also notice that position $\HypQ[3]$ 
has a question mark. 
	
We investigate now what can happen with $\HypQ[3]$.
Firstly, note that because $\HypQ[8] = x_8$ which is persisted before $c_k$, the enqueue
operations that are active in $E_k$ are at least up to $\var{enq}_8$.
In $\HypQ[3]$ there are two possible scenarios, either we have an $\var{enq}_3$ with a successful
\Call{CAS2}{}, or not.
Let $\var{enq}_3$ be an enqueue operation that had successfully inserted its item $x'$.
Because we have $\HypQ[8] = x_8$, item $x'$ must have been removed in order for $\var{enq}_8$ to
successfully insert its item $x_8$ in $\crqVar.\Q[3]$ and be written back to NVM.
Therefore, there was also a $\var{deq}_3$ that removed successfully and returned $x'$.
Because $\var{deq}_3$ returns successfully, it has to be assigned a linearization point.
If we linearize $\var{deq}_3$ we have to also linearize $\var{deq}_0$, $\var{deq}_1$, and 
$\var{deq}_2$. If we do not, then we violate durable linearizability.
This gives us a lower bound for $\crqVar.\Head \geq 4$.
If there was no $\var{enq}_3$ and $\var{enq}_8$ reached $\crqVar.\Q[3]$ early, and the \CAS\ at
line~\ref{pcrq:eqcas} was successful, $x_4$ is inserted. It is also written back in order to be
visible at recovery time. But there were no dequeue operations, and thus \crqVar.\Head should
be equal to $0$.

The problem is that there is no information for the recovery function to correctly choose a value
for \Head.
The two scenarios above are indistinguishable, because they give the same state of $\crqVar.\Q$
array after $c_k$.
\end{scenario}
}
\remove{
\begin{scenario} \label{scn:persistEmpty}
\begin{figure}[htb]
	\centering
	\includegraphics[width=0.65\textwidth]{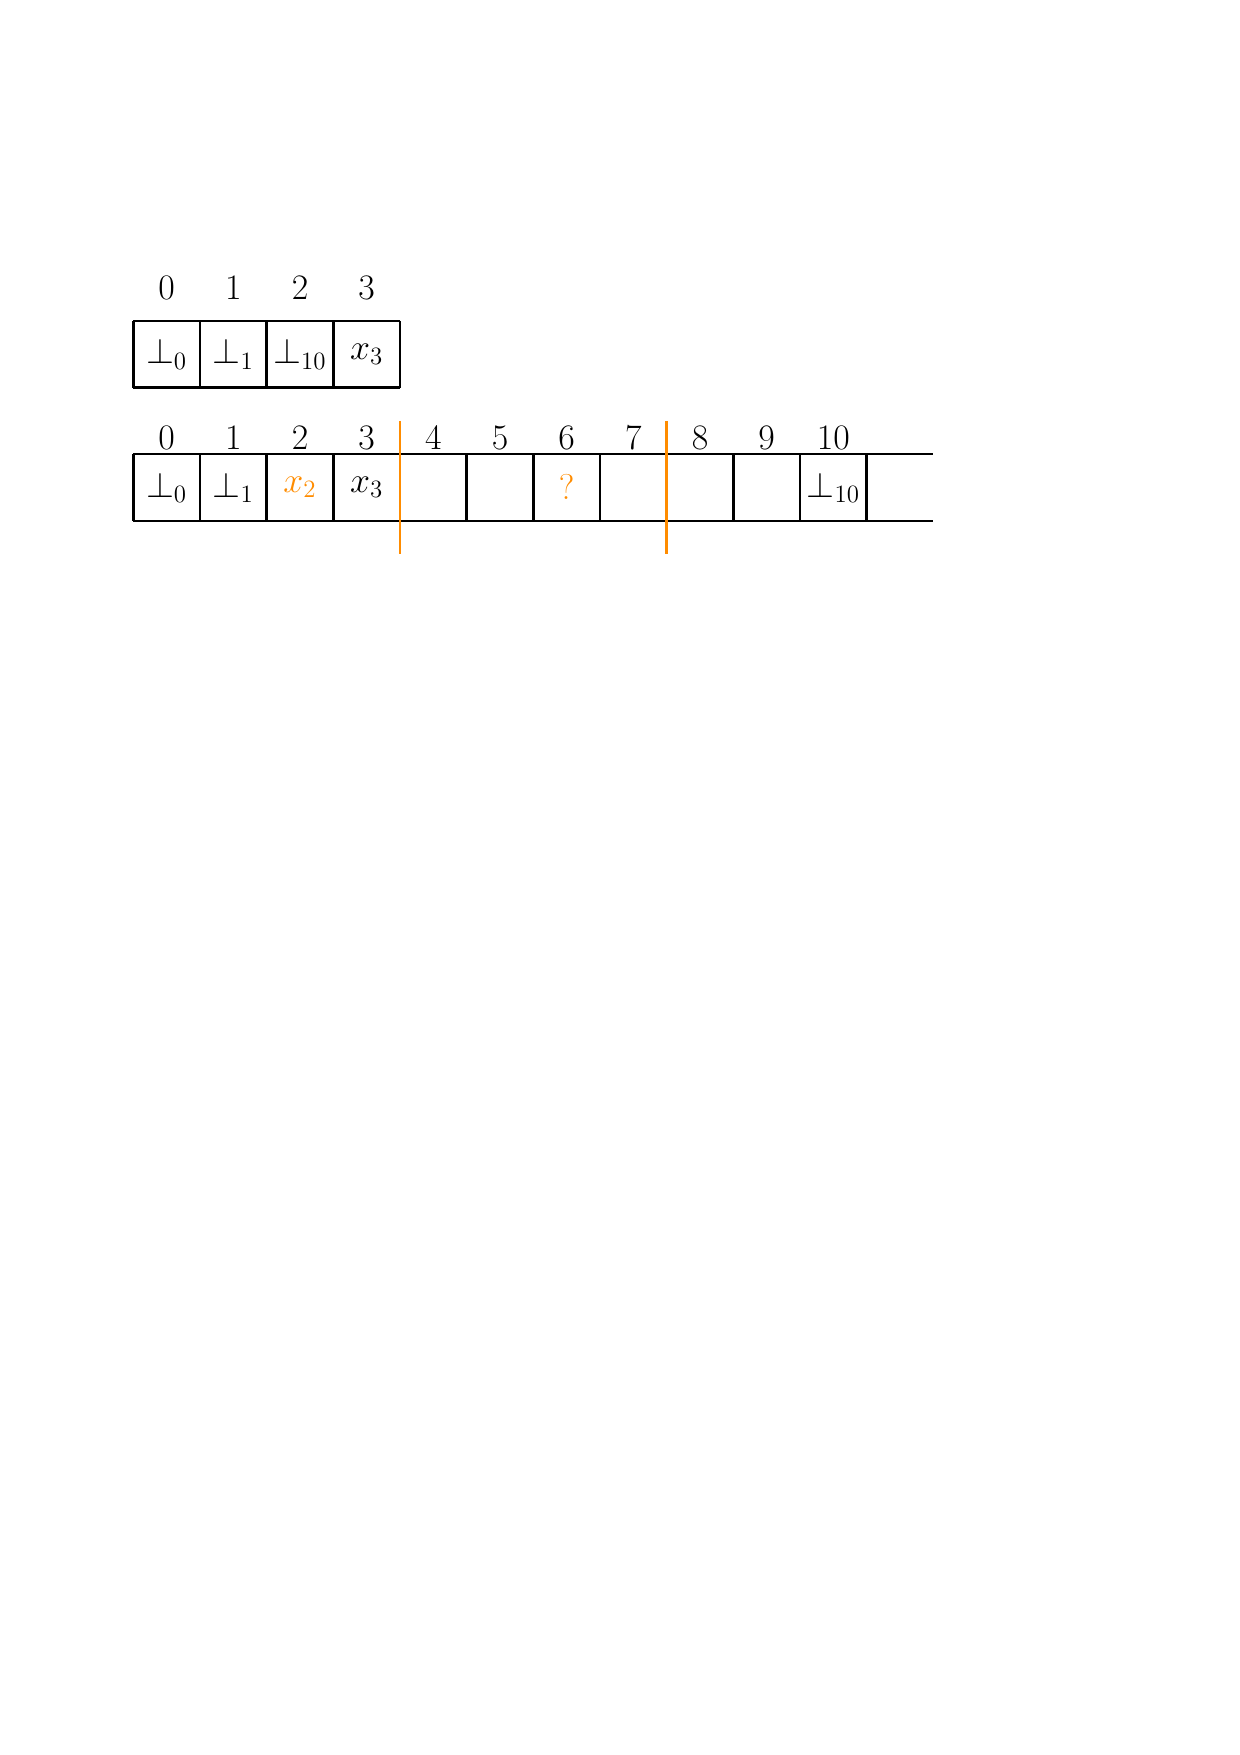}
	\caption{State of the circular array for the example justifying the need of the pair of \pwbi-\psynci\ of 
	lines~\ref{pcrq:dqpwbHead2}-\ref{pcrq:dqpsyncHead2} and the hypothetical infinite array bellow.
	Note that the subscripts at each item corresponds to the value of its index field.} 
	\label{fig:emptyExample}
\end{figure}

Consider a circular array of size $4$. At first we have four enqueue operations, 
$\var{enq}_0, \ldots, \var{enq}_3$, that begin their execution. 
Operations $\var{enq}_2$ and $\var{enq}_3$ finish their execution inserting 
successfully their items, $x_2$ and $x_3$ respectively, and returning \OK. Now we have three 
dequeue operations, $\var{deq}_0$ through $\var{deq}_2$, which begin their execution. Operation 
$\var{deq}_2$ successfully removes and returns $x_2$. Since the value of \Head\ is already $3$ 
when $\var{deq}_2$ persists it, $\Head = 3$ is successfully written 
back to NVM by $\var{deq}_2$. Now four more dequeue operations, $\var{deq}_3$ through 
$\var{deq}_6$, begin their execution, and $\var{deq}_6$ performs an empty transition. Because at 
this point $\Head{} = 7$ and $\Tail{} = 4$, $\var{deq}_6$ returns \EMPTY. Notice that operations 
$\var{enq}_2$, $\var{enq}_3$, $\var{deq}_2$, and $\var{deq}_6$ have returned and thus must be 
assigned a linearization point.

Now there is a failure and the last persisted value of \Head\ before the crash was 
$3$.
The state of the queue at recovery time is $(1,0,\bot)$, $(1,1,\bot)$, $(1,10,\bot)$, $(1,3,x_3)$ 
and is shown in Figure~\ref{fig:emptyExample}.
At recovery time we get $\Head=3$ and $\Tail=7$ (based on the execution of the recovery function 
in Algorithm~\ref{alg:pcrq}), which results in a state of the queue that is not empty. The 
problem is that we have assigned a linearization point to a dequeue operation that returned 
\EMPTY, but at recovery we have a non-empty queue.
\end{scenario}

\begin{scenario} \label{scn:pcrq-deq-persists}
\begin{figure}[htb]
	\centering
	\includegraphics[width=0.35\textwidth]{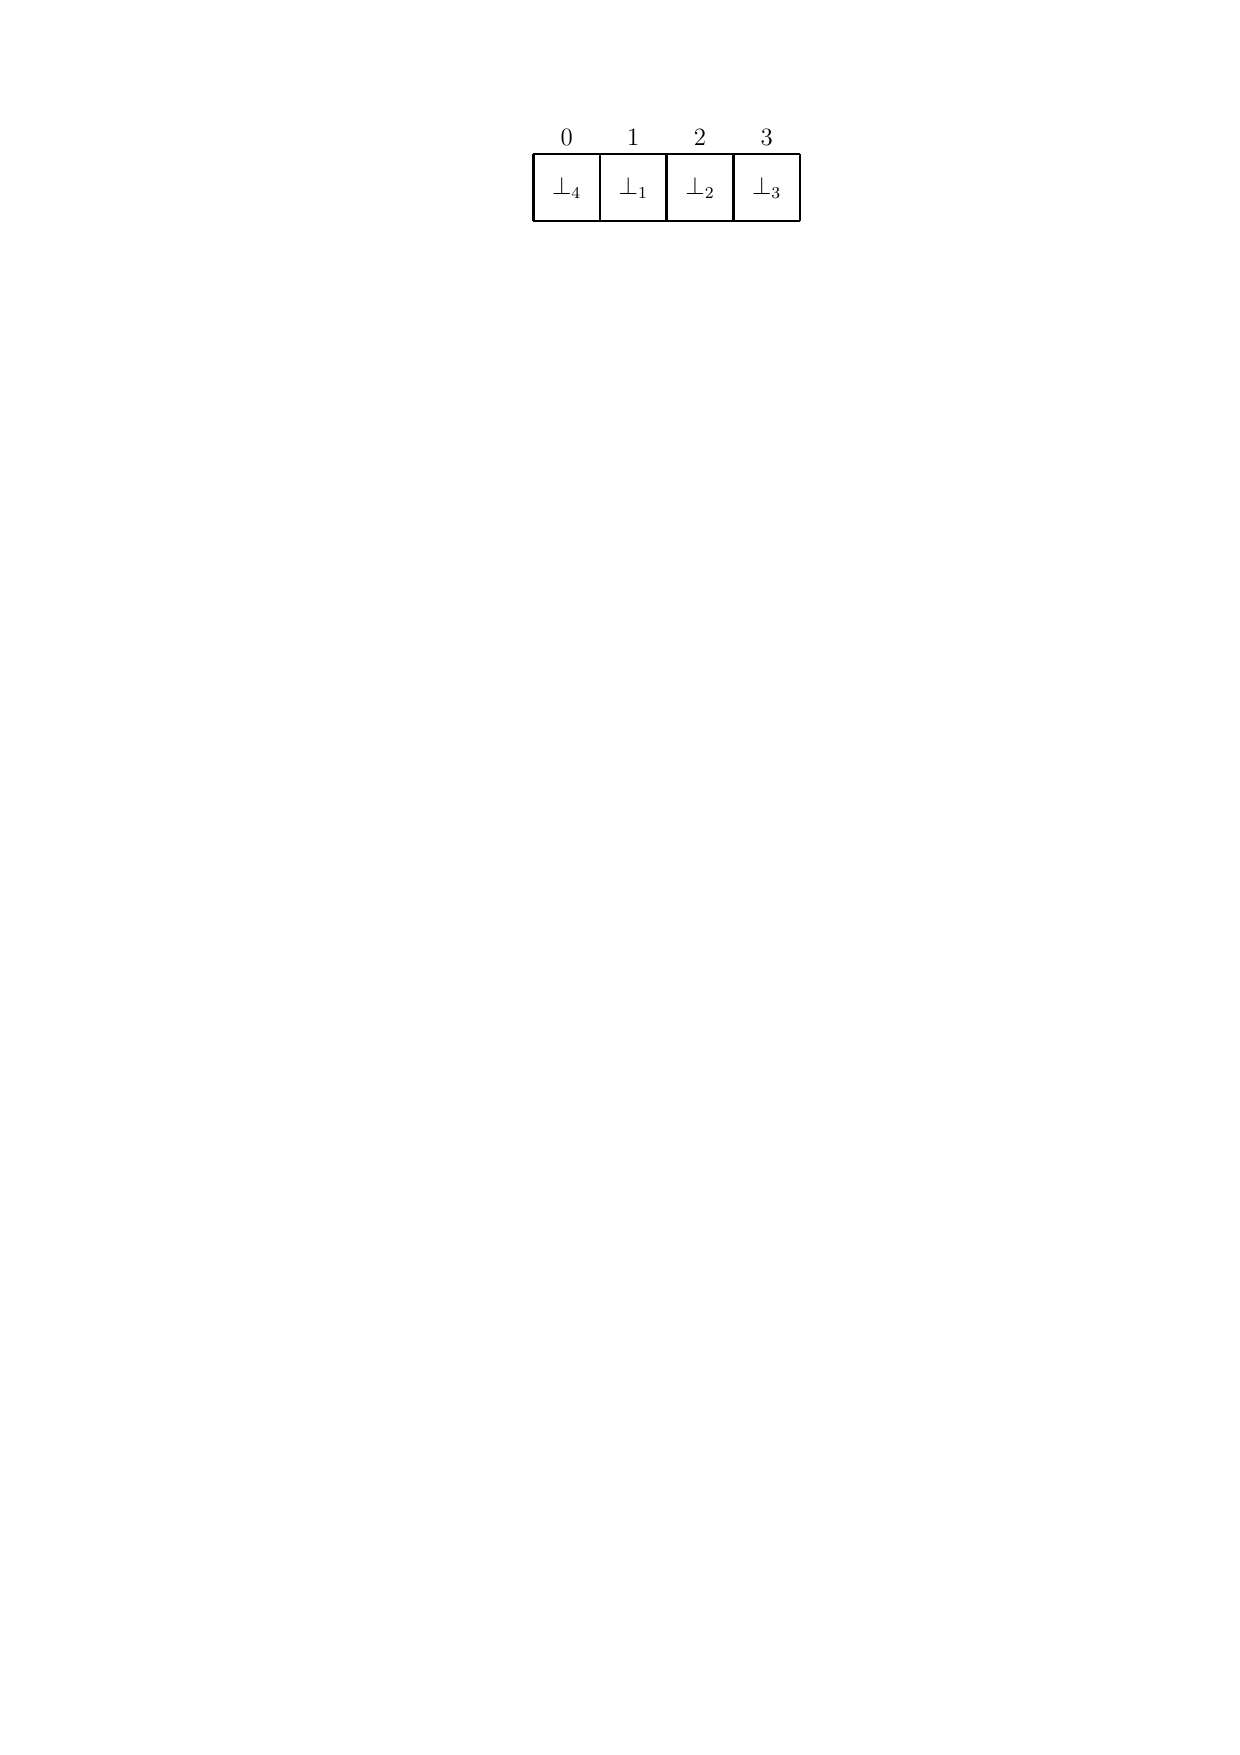}
	\caption{The circular array state for Scenario~\ref{scn:pcrq-deq-persists}. Note that the
	subscript of each item corresponds to the value of its index field.}
\end{figure}
Let $R=4$ be the size of the circular array $\crqVar.\Q$. Consider the following execution.
Initially there are three enqueue operations $\var{enq}_0(x_0)$, $\var{enq}_1(x_1)$, and 
$\var{enq}_2(x_2)$. Operation $\var{enq}_0(x_0)$ inserts its item and returns \OK, operation
$\var{enq}_1(x_1)$ executes its \FAI\ of line~\ref{pcrq:eqfaa} and sleeps, and operation
$\var{enq}_2(x_2)$ executes its \CAS\ of line~\ref{pcrq:eqcas} successfully and sleeps.
Now three dequeue operations become active $\var{deq}_0()$, $\var{deq}_1()$, and $\var{deq}_2()$.
Operations $\var{deq}_0()$ and $\var{deq}_1()$ execute only their \FAI\ on \Head\ and then sleep,
while $\var{deq}_2()$ executes its \CAS\ of line~\ref{pcrq:dqtran} successfully removing $x_2$ 
and then sleeps.
At this point $\Head = 3$ and $\Tail = 3$.
Now operation $\var{enq}_2(x_2)$ wakes up 
and returns \OK, and because of the pair of \pwbi-\psynci\ of lines~\ref{pcrq:eqpwb}-\ref{pcrq:eqpsync},
$\crqVar.\Q[2]$ (which contains the triplet $\langle s, 6, \bot \rangle$) is written back to NVM
(this write-back could have also occurred by the system by evicting the appropriate cache line).
Lastly, there are five more enqueue operations $\var{enq}_3(x_3)$ through $\var{enq}_7(x_7)$.
Operations $\var{enq}_3(x_3)$ through $\var{enq}_6(x_6)$ execute their \FAI\ on \Tail\ and then
sleep. Operation $\var{enq}_7(x_7)$ inserts successfully $x_7$ and returns \OK.
At this point $\Head = 3$ and $\Tail = 8$, none of them is persisted and a system-wide failure
occurs. The operations that we must assign linearization points are these that have successfully
returned before the occurrence of the crash. The question is what we should do with 
$\var{deq}_2()$, because \Head\ is not persisted but its removal of $x_2$ is persisted.
If we do not linearize it and, at recovery time, choose $\Head = 0$, after the crash there is no
way to dequeue $x_2$, which violates durable linearizability. Therefore we have to take into
consideration the triplets that are persisted. \qed
\end{scenario}

\begin{scenario} \label{scn:pcrq-rec-max}
\begin{figure}[htb]
	\centering
	\includegraphics[width=0.4\linewidth]{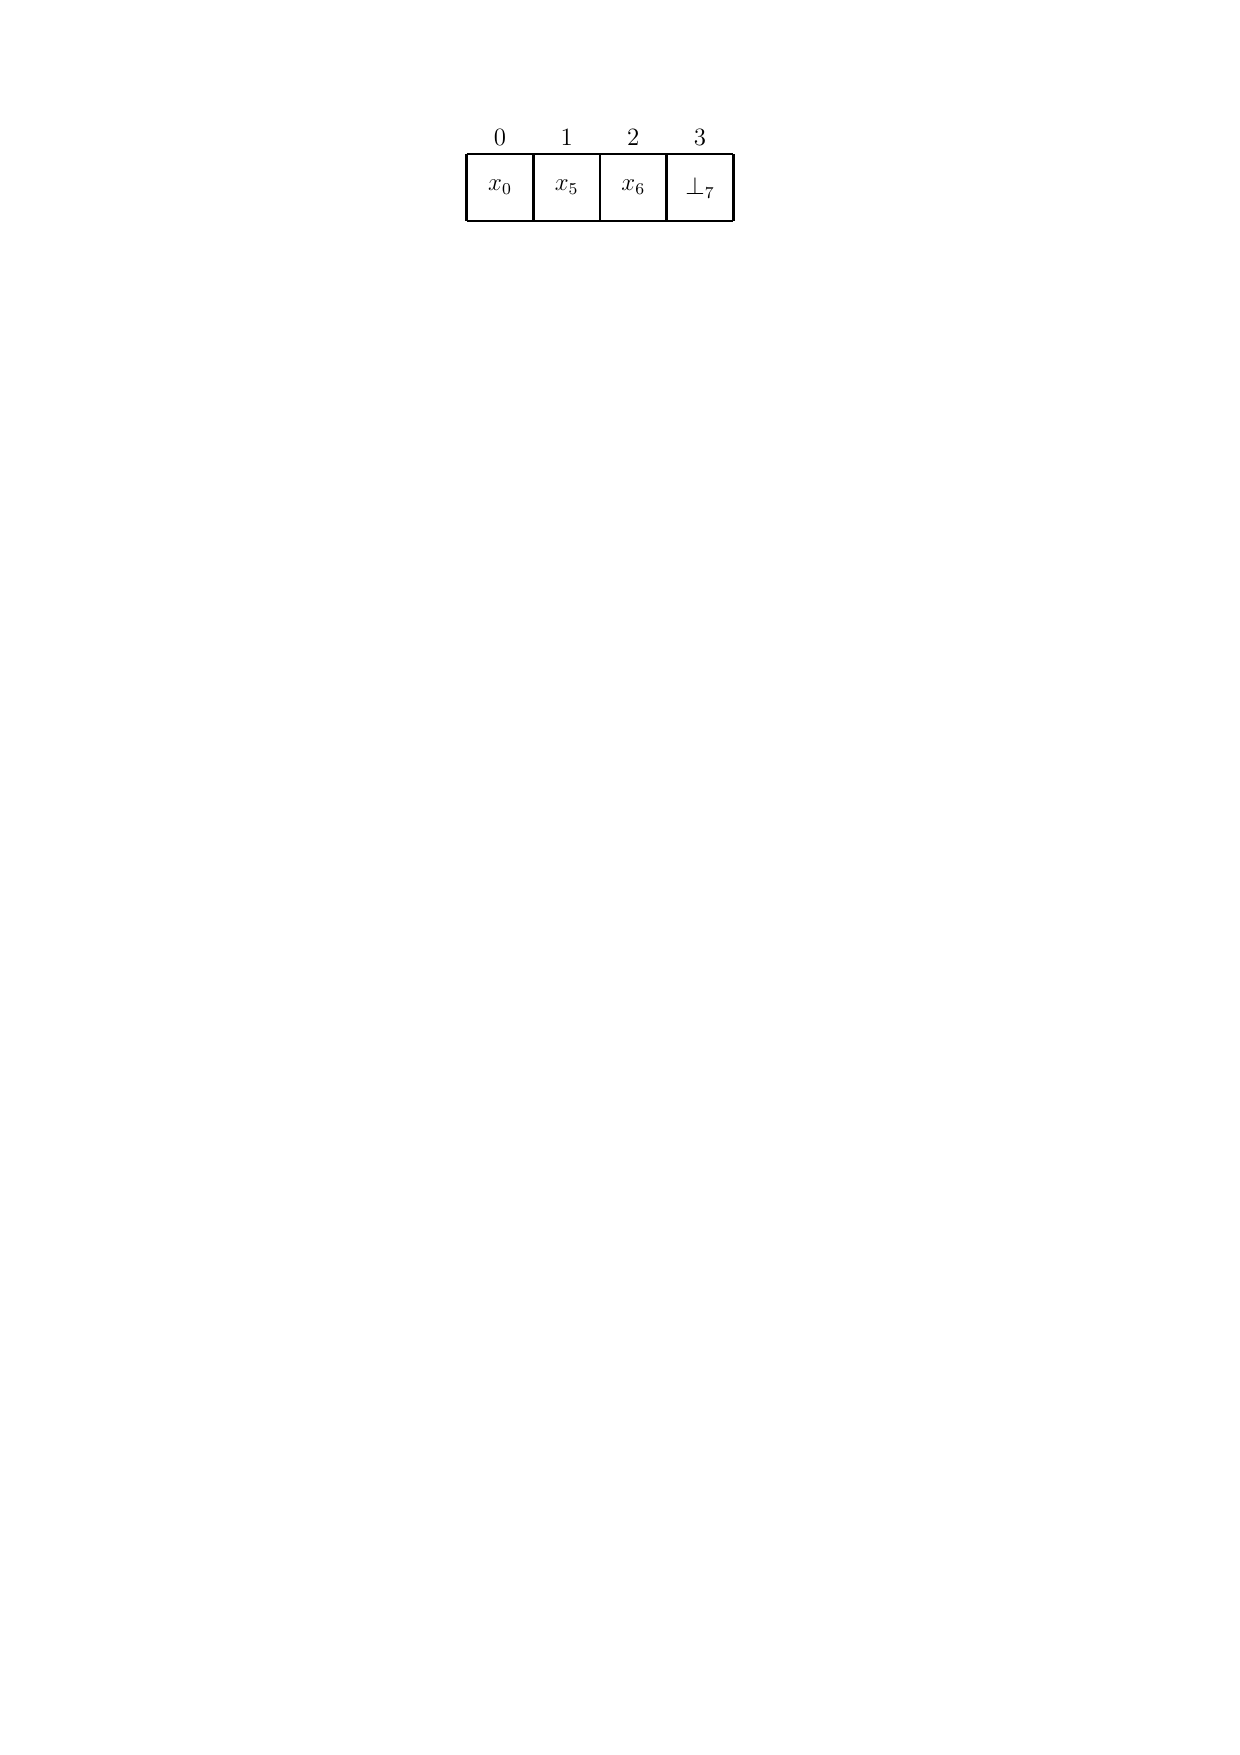}
	\caption{Circular array state to justify the movement of \Head\ based on the minimum occupied
	node.} \label{fig:movehead}
\end{figure}

Let the state of the circular array after executing lines 
\ref{pcrq:recinimax}-\ref{pcrq:recsetmax} of the recovery function of 
Algorithm~\ref{alg:pcrq} be the one shown in Figure~\ref{fig:movehead}, 
where $R = 5$. Note that $\Head = 10$ after executing lines 
\ref{pcrq:recinimax}-\ref{pcrq:recsetmax}. As explained later we 
will linearize all dequeue operations with indices up until $9$. However, \Head\ points to an element 
with index $5$ which is less than $9$. Since the dequeue with index $5$ will have already been 
linearized by the crash, \Head\ is updated to the smallest index of an occupied position, which is 
larger than $10$. \qed

\remove{Note that $\Tail = 13$ because of a triplet $\langle s, 12, x_{12}\rangle$ at 
$\Q[2]$, and $\Head = 10$ because of a triplet $\langle s, 9, \bot\rangle$ at $\Q[4]$. As discussed 
previously we have to take into consideration unoccupied nodes for both \Head\ and \Tail.
Let the minimum index of an occupied node, larger than \Head, be $11$. This is possible if at position 
$\Head \bmod R = 0$ there is a triplet $\langle s, 5, x_5\rangle$, where $x_5$ can be any value (even
$\bot$).}
\end{scenario}
}

\begin{figure}[ht]
	\includegraphics[width=\textwidth]{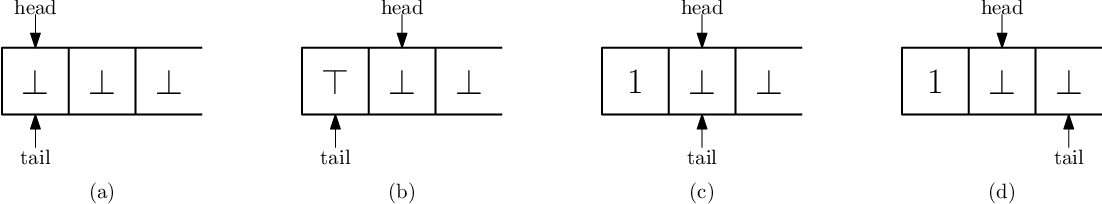}
	\caption{Livelock example for the \textit{infinite} queue.}\label{fig:iqlivelock}
	\end{figure}
	
	\begin{scenario} \label{scn:livelock}
	One process executes \Call{Enqueue}{1} and another process executes \Call{Dequeue}{} concurrently. 
	At first the dequeue operation executes lines \ref{piq:dqfaa} and \ref{piq:dqswap}, changing \Head{} 
	to point to the next cell and inserting $\top$ to the first cell, the state is now shown in
	Figure~\ref{fig:iqlivelock}~(b). 
	Then the enqueue operation reads \Tail{} and changes it to point to the next cell 
	(line~\ref{piq:faa}). 
	It inserts number $1$ to the first cell (line~\ref{piq:swap}) and the state now is as shown in
	Figure~\ref{fig:iqlivelock}~(c). 
	Since the \Call{Get\&Set}{} of line~\ref{piq:swap} returns $\top$, the enqueue operation starts
	another loop (line~\ref{piq:loop}). 
	It executes line~\ref{piq:faa} and now the state is 
	as shown on Figure~\ref{fig:iqlivelock}~(d). From there the two conditions in 
	lines \ref{piq:botcheck} and \ref{piq:dqempty} 
	of the dequeue operation are false and we continue the same way, forever, without any of the two 
	processes successfully returning something.
	\end{scenario}

\section{Algorithms} \label{sec:algos}

We provide an enhanced version of the \PIQ\ pseudocode, 
in which we periodically write back \Tail\ to reduce the performance 
cost of the recovery function.

% \input{main_algo/per_lcrq_code}

% \begin{algorithm}
% \caption{Helper function for fixing the queue state}\label{alg:fix}
% \begin{algorithmic}[1]
% \Function{FixState}{crq}
% 	\While{True}
% 		\State $h\gets$ \Call{Fetch\&Add}{crq.head, 0}
% 		\State $t\gets$ \Call{Fetch\&Add}{crq.tail, 0}
% 		\If{$\text{crq.tail}\neq t$}
% 			\State \textbf{continue}
% 		\EndIf
% 		\If{$h\leq t$}
% 			\State \Return
% 		\EndIf
% 		\If{$\Call{CAS}{\text{crq.tail}, t, h}$}
% 			\State \Return
% 		\EndIf
% 	\EndWhile
% \EndFunction
% \end{algorithmic}
% \end{algorithm}

% \section{The problem in distinguishing between empty and normal dequeue transitions}

% \begin{figure}[h]
% 	\centering
% 	\includegraphics[width=0.8\textwidth]{fig/per_crq_uncertainty_example_complex.pdf}
% 	\caption{Complicated \CRQ{} uncertainty example}
% 	\label{fig:crqcompunc}
% \end{figure}
\end{subappendices}
